# Supplementary material for: DVM: Towards Controllable LLM Agents in Social Deduction Games
Source: arXiv:2501.06695 source file (2025-01-12)
Supplement: Supplementary file 1 [file appendix.tex]

\section{Appendix}

\subsection{Decision Chain}
\label{sub:decision_chain}
we demonstrate some examples of decision chain of human players. Each item includes decision chain, win rate and its game count.

\textbf{Werewolf}: 
\begin{description}
    \item[kill: villager vote: seer kill: witch vote: hunter 0.98 (971)]
    \item[kill: villager vote: seer kill: witch vote: pass 
 0.63 (932)]
    \item[kill: villager kill: werewolf 0.00 (312)]
\end{description}

\textbf{Villager}:
\begin{description}
    \item[vote: werewolf vote: werewolf vote: werewolf 0.95 (687)]
    \item[vote: werewolf vote: hunter 0.44 (556)]
    \item[vote: seer vote: villager vote: pass 0.13 (684)]
\end{description}

\textbf{Seer}:
\begin{description}
    \item[check: werewolf vote: werewolf check: werewolf vote: pass 0.77 (413)]
    \item[check: villager vote: werewolf check: werewolf vote: pass 0.65 (493)]
    \item[check: werewolf vote: werewolf check: pass vote: pass 0.04 (539)]
\end{description}

\textbf{Witch}
\begin{description}
    \item[antidote: villager vote: werewolf poison: werewolf vote: werewolf
        0.98 (317)]
    \item[antidote: villager vote: werewolf poison: villager vote: pass vote: pass 
        0.52 (270)]
    \item[antidote: villager vote: seer poison: villager vote: pass 
        0.00 (263)]
\end{description}

\textbf{Hunter}:
\begin{description}
    \item[vote: werewolf vote: none shot: werewolf 
        0.92 (306)]
    \item[vote: werewolf vote: none shot: werewolf vote: none 
        0.51 (105)]
    \item[vote: none vote: werewolf shot: witch 
        0.0 (107)]
\end{description}
% Optionally include supplemental material (complete proofs, additional experiments and plots) in appendix.
% All such materials \textbf{SHOULD be included in the main submission.}

%%%%%%%%%%%%%%%%%%%%%%%%%%%%%%%%%%%%%%%%%%%%%%%%%%%%%%%%%%%%

\newpage
